# Supplementary material for: Enantioselective Topological Frequency Conversion
Source: arXiv:2105.05469 source file (2022-03-05)
Supplement: Supplementary file 1 [file supporting_information_3_4_22.pdf]

# Enantioselective Topological Frequency Conversion

Kai Schwennicke and Joel Yuen-Zhou*

*Department of Chemistry and Biochemistry, University of California, San Diego, La Jolla, California 92093, United States*

E-mail: joelyuen@ucsd.edu

## 1 Rotational eigenstates

Here we present the low angular momentum eigenstates of the asymmetric top. For completeness, we reintroduce the asymmetric top Hamiltonian

$$H_0 = AJ_a^2 + BJ_b^2 + CJ_c^2, \tag{1}$$

where $J_a$, $J_b$, $J_c$ are the angular momentum operators with respect to the principal axes $\hat{\boldsymbol{a}}$, $\hat{\boldsymbol{b}}$, $\hat{\boldsymbol{c}}$, and $A > B > C$ are the corresponding rotational constants. The $B = C$ case corresponds to a prolate top with eigenstates labeled $|J, K, M\rangle$, where $J = 0, 1, 2...$ is the rotational quantum number and $M, K = -J, -J+1, -J+2, ..., J$ are the quantum numbers that characterize the projection of the total angular momentum along the $a$-principal axis and $z$-laboratory-fixed axis. The eigenstates of the asymmetric top Hamiltonian can be

expressed as superpositions of the prolate top eigenstates as follows:

$$|J,\tau,M\rangle = \sum_K A_K^{J,M}(\tau)|J,K,M\rangle. \tag{2}$$

Note that the quantum numbers $J$, $M$ are conserved by $H_0$, and $\tau$ serves as the quantum number to differentiate between states with the same $J$ and $M$. The eigenstates of Eq. 1 with a rotational quantum number of $J = 0$ or $J = 1$ are

$$\begin{aligned}
|0,\tau=1,0\rangle &\equiv |0,K=0,0\rangle, \\
|1,\tau=1,M\rangle &\equiv |1,K=0,M\rangle, \\
|1,\tau=2,M\rangle &\equiv \frac{1}{\sqrt{2}}|1,K=1,M\rangle - \frac{1}{\sqrt{2}}|1,K=-1,M\rangle, \\
|1,\tau=3,M\rangle &\equiv \frac{1}{\sqrt{2}}|1,K=1,M\rangle + \frac{1}{\sqrt{2}}|1,K=-1,M\rangle,
\end{aligned} \tag{3}$$

where $M = -1, 0, 1$[1]. In the main text, we do not couple the states $|1,\tau=1,M\rangle$ to others, and thus ignore them.

# 2 Change of Basis

We present the necessary change of basis to obtain the effective Hamiltonian presented in Eq. 8 in the main text. We first introduce $|2,B\rangle = \frac{1}{\sqrt{2}}(|2,1\rangle + |2,-1\rangle)$ and $|2,D\rangle = \frac{1}{\sqrt{2}}(|2,1\rangle - |2,-1\rangle)$, which we refer to as the "bright" and "dark" state respectively. It is easy to see that bright state couples to $|1,0\rangle$ and $|3,0\rangle$, while the dark state is uncoupled (see Eq. 7). Ignoring the dark state, the Hamiltonian in the rotating frame becomes

$$\mathcal{H}^{R,S}(t) = \frac{1}{2}\begin{pmatrix} -2\hbar\delta & -\frac{\mu_b^{R,S}}{\sqrt{3}}\mathcal{E}_{21}(t) & -\frac{i\mu_c^{R,S}}{\sqrt{3}}\mathcal{E}_{31}(t) \\ -\frac{\mu_b^{R,S}}{\sqrt{3}}\mathcal{E}_{21}(t) & 0 & -\frac{\mu_a^{R,S}}{2}\mathcal{E}_{32}(t) \\ \frac{i\mu_c^{R,S}}{\sqrt{3}}\mathcal{E}_{31}(t) & -\frac{\mu_a^{R,S}}{2}\mathcal{E}_{32}(t) & 2\hbar\delta \end{pmatrix} \tag{4}$$

In the complex basis $|+\Pi\rangle, |0\rangle, |-\Pi\rangle$, where $|\pm\Pi\rangle = \frac{1}{\sqrt{2}}(|1,0\rangle \pm i|3,0\rangle)$ and $|0\rangle = |2,B\rangle$, Eq. 4 becomes

$$\mathcal{H}^{R,S}(t) = -\frac{\mu_b^{R,S}\mathcal{E}_{21}(t)}{2\sqrt{3}\hbar}L_x - \frac{\mu_a^{R,S}\mathcal{E}_{32}(t)}{4\hbar}L_y + \frac{\mu_c^{R,S}\mathcal{E}_{31}(t)}{2\sqrt{3}\hbar}L_z - \frac{\delta}{2\hbar}(L_+^2 + L_-^2) \tag{5}$$

where $L_x = \frac{\hbar}{\sqrt{2}}\begin{pmatrix}0 & 1 & 0\\ 1 & 0 & 1\\ 0 & 1 & 0\end{pmatrix}$, $L_y = \frac{\hbar}{\sqrt{2}}\begin{pmatrix}0 & -i & 0\\ i & 0 & -i\\ 0 & i & 0\end{pmatrix}$, $L_z = \hbar\begin{pmatrix}1 & 0 & 0\\ 0 & 0 & 0\\ 0 & 0 & -1\end{pmatrix}$ are the angular momentum operators for a spin-1 particle and $L_+ = \hbar\sqrt{2}\begin{pmatrix}0 & 1 & 0\\ 0 & 0 & 1\\ 0 & 0 & 0\end{pmatrix}$, $L_- = \hbar\sqrt{2}\begin{pmatrix}0 & 0 & 0\\ 1 & 0 & 0\\ 0 & 1 & 0\end{pmatrix}$ are the corresponding ladder operators. Eq. 5 is the effective Hamiltonian used to study the topology of the system presented in the main text.

# 3 Adiabatic perturbation theory

For completeness, we briefly review adiabatic perturbation theory. Let $|\tilde{\psi}(t)\rangle = \sum_l \tilde{c}_l(t)|\epsilon_l(t)\rangle$ be the solution of the time-dependent Schrödinger equation (TDSE) $i\hbar\partial_t|\tilde{\psi}(t)\rangle = \mathcal{H}(t)|\tilde{\psi}(t)\rangle$, where $\{|\epsilon_l(t)\rangle\}$ are the adiabatic eigenstates satisfying $\mathcal{H}(t)|\epsilon_l(t)\rangle = \epsilon_l(t)|\epsilon_l(t)\rangle$. Employing the TDSE, the following differential equation is obtained for $\tilde{c}_l(t)$,

$$i\hbar\partial_t\tilde{c}_l(t) = \epsilon_l(t)\tilde{c}_l(t) - i\hbar\sum_{l'}\langle\epsilon_l(t)|\boldsymbol{\omega}\cdot\nabla_{\boldsymbol{\omega}t}|\epsilon_{l'}(t)\rangle\tilde{c}_{l'}(t), \tag{6}$$

where $\boldsymbol{\omega} = (\omega_1, \omega_2)$. Ignoring non-adiabatic terms in Eq. 6 for $l' \neq l$,

$$\tilde{c}_l(t) \approx \tilde{c}_l(0)e^{-i\int_0^t dt'[\epsilon_l(t') - i\hbar\langle\epsilon_l(t')|\boldsymbol{\omega}\cdot\nabla_{\boldsymbol{\omega}t}|\epsilon_l(t')\rangle]/\hbar}. \tag{7}$$

Hereafter, we assume that the system is initialized in the $l-$th adiabatic state $|\tilde{\psi}(0)\rangle = |\epsilon_l(0)\rangle$. Eq. 7 is a statement of the adiabatic theorem and implies that the system shall remain in the $l-$th adiabatic state, $|\tilde{\psi}(t)\rangle \approx$ (phase factor) $\times\, |\epsilon_l(t)\rangle$.

However, we are interested in $O(\hbar\omega)$ non-adiabatic corrections to Eq. 7. We rewrite $\tilde{c}_{l'} = \hbar\boldsymbol{\omega}\tilde{c}_l(t)a_{l'}(t)$ for $l' \neq l$,

$$|\tilde{\psi}(t)\rangle = \tilde{c}_l(t)[|\epsilon_l(t)\rangle + \sum_{l'\neq l}\hbar\boldsymbol{\omega}a_{l'}(t)|\epsilon_{l'}(t)\rangle], \tag{8}$$

and insert this ansatz into Eq. 6,

$$\epsilon_l(t)\tilde{c}_l(t)a_{l'}(t)\hbar\boldsymbol{\omega} + O(\hbar^2\boldsymbol{\omega}^2) = \hbar\boldsymbol{\omega}\epsilon_{l'}(t)\tilde{c}_l(t)a_{l'}(t) - i\hbar\langle\epsilon_{l'}(t)|\boldsymbol{\omega}\cdot\nabla_{\boldsymbol{\omega}t}|\epsilon_l(t)\rangle\tilde{c}_l(t) + O(\hbar^2\boldsymbol{\omega}^2), \tag{9}$$

where we used $\partial_t a_{l'}(t) = \hbar\boldsymbol{\omega}\cdot\nabla_{\omega t}a_{l'}(t)$. Solving for $a_{l'}(t)$, the $O(\hbar\omega)$ wavefunction is,

$$|\tilde{\psi}(t)\rangle = \tilde{c}_l(t)\left[|\epsilon_l(t)\rangle - i\hbar\sum_{l'\neq l}\frac{|\epsilon_{l'}(t)\rangle\langle\epsilon_{l'}(t)|\boldsymbol{\omega}\cdot\nabla_{\boldsymbol{\omega}t}|\epsilon_l(t)\rangle}{\epsilon_l(t)-\epsilon_{l'}(t)}\right]. \tag{10}$$

**Calculating $\mathcal{P}_{av}(\omega_1)$ and $\mathcal{P}_{av}(\omega_2)$**

Here, $\langle\tilde{\psi}(t)|\partial_{\omega_i t}\mathcal{H}(t)|\tilde{\psi}(t)\rangle$ and $P_{av}(\omega_i)$ are derived when the system is initiated in the adiabatic state $|\epsilon_l(0)\rangle$ and evolved near the adiabatic limit. Employing Eq. 10 for $|\tilde{\psi}(t)\rangle$, and making the change of variables $(\omega_1 t, \omega_2 t) = (\theta_1, \theta_2)$, the following expression to $O(\hbar\omega)$ is obtained:

$$\begin{aligned}\langle\tilde{\psi}(t)|\nabla_{\boldsymbol{\omega}t}\mathcal{H}(t)|\tilde{\psi}(t)\rangle &= \langle\epsilon_l(\boldsymbol{\theta})|\nabla_{\boldsymbol{\theta}}\mathcal{H}(\boldsymbol{\theta})|\epsilon_l(\boldsymbol{\theta})\rangle - \Big\{i\hbar\sum_{l'\neq l}\frac{\langle\epsilon_l(\boldsymbol{\theta})|\nabla_{\boldsymbol{\theta}}\mathcal{H}(\boldsymbol{\theta})|\epsilon_{l'}(\boldsymbol{\theta})\rangle\langle\epsilon_{l'}(\boldsymbol{\theta})|\boldsymbol{\omega}\cdot\nabla_{\boldsymbol{\theta}}|\epsilon_l(\boldsymbol{\theta})\rangle}{\epsilon_l(\boldsymbol{\theta})-\epsilon_{l'}(\boldsymbol{\theta})} + \text{h.c}\Big\}\\ &= \nabla_{\boldsymbol{\theta}}\epsilon_l(\boldsymbol{\theta}) - \Big\{i\hbar\langle\nabla_{\boldsymbol{\theta}}\epsilon_l(\boldsymbol{\theta})|\boldsymbol{\omega}\cdot\nabla_{\boldsymbol{\theta}}|\epsilon_l(\boldsymbol{\theta})\rangle + \text{h.c}]\Big\}\\ &= \nabla_{\boldsymbol{\theta}}\epsilon_l(\boldsymbol{\theta}) - \hbar\boldsymbol{\omega}\times\hat{\boldsymbol{v}}_\perp F_l(\boldsymbol{\theta}),\end{aligned} \tag{11}$$

where $\boldsymbol{\omega}\times\hat{\boldsymbol{v}}_\perp = (\omega_2, -\omega_1)$ and $F_l(\boldsymbol{\theta}) = i\langle\partial_{\theta_1}\epsilon_l(\boldsymbol{\theta})|\partial_{\theta_2}\epsilon_l(\boldsymbol{\theta})\rangle + \text{h.c.}$ is the Berry curvature of

the $l-$th band.

## 4 Analytical evaluation of Chern numbers

Here, we analytically compute the Chern numbers for the bands of the system in the main text when $\delta = 0$. We follow the procedure described in[2]. We first consider the three-level Hamiltonian:

$$\mathcal{H}(\boldsymbol{\theta}) = \sum_{s=\pm1} sh_3(\boldsymbol{\theta})|s\rangle\langle s| + \Big\{[h_1(\boldsymbol{\theta}) - ish_2(\boldsymbol{\theta})]|s\rangle\langle 0| + \text{h.c.}\Big\}, \tag{12}$$

where $h_1(\boldsymbol{\theta})$, $h_2(\boldsymbol{\theta})$, $h_3(\boldsymbol{\theta})$ are real valued. Next, we invoke the unitary transformation $U(\boldsymbol{\theta}) = \sum_{s=0,\pm1} e^{is\alpha(\boldsymbol{\theta})}|s\rangle\langle s|$, such that $\tan\alpha(\boldsymbol{\theta}) = h_2(\boldsymbol{\theta})/h_1(\boldsymbol{\theta})$, to define the real valued Hamiltonian,

$$\begin{aligned}\mathcal{H}'(\boldsymbol{\theta}) &= U(\boldsymbol{\theta})\mathcal{H}(\boldsymbol{\theta})U^\dagger(\boldsymbol{\theta}) \\ &= \sum_{s=\pm1} sh_3(\boldsymbol{\theta})|s\rangle\langle s| + \sqrt{h_1^2(\boldsymbol{\theta}) + h_2^2(\boldsymbol{\theta})}(|s\rangle\langle 0| + \text{h.c.}).\end{aligned} \tag{13}$$

A set of eigenstates for $\mathcal{H}'(\boldsymbol{\theta})$ can be defined as $|\epsilon_l'(\boldsymbol{\theta})\rangle = \sum_{s=0,\pm1} c_{l,s}(\boldsymbol{\theta})|s\rangle$, where the coefficients $c_{l,s}(\boldsymbol{\theta})$ are real. The eigenstates of $\mathcal{H}(\boldsymbol{\theta})$ are

$$|\epsilon_l(\boldsymbol{\theta})\rangle = U^\dagger(\boldsymbol{\theta})|\epsilon_l'(\boldsymbol{\theta})\rangle = \sum_{s=0,\pm1} c_{l,s}(\boldsymbol{\theta})e^{-is\alpha(\boldsymbol{\theta})}|s\rangle. \tag{14}$$

The Berry connection for the $l-$th band is

$$\begin{aligned}\boldsymbol{A}_l(\boldsymbol{\theta}) &= i\langle\epsilon_l(\boldsymbol{\theta})|\nabla_{\boldsymbol{\theta}}|\epsilon_l(\boldsymbol{\theta})\rangle \\ &= \nabla_{\boldsymbol{\theta}}\alpha(\boldsymbol{\theta})\sum_{s=\pm1} sc_{l,s}^2(\boldsymbol{\theta}),\end{aligned} \tag{15}$$

where we used the fact that $\sum_{s=0,\pm1} c_{l,s}(\boldsymbol{\theta})\nabla_{\boldsymbol{\theta}} c_{l,s}(\boldsymbol{\theta}) = \frac{1}{2}\nabla_{\boldsymbol{\theta}} \sum_{s=0,\pm1} |c_{l,s}|^2 = 0$. The Berry curvature is defined as the $z$-component of the curl of the Berry connection, *i.e.*, $F_l(\boldsymbol{\theta}) = (\nabla_{\boldsymbol{\theta}} \times \boldsymbol{A}_l(\boldsymbol{\theta})) \cdot \hat{z}$. Note that there are singularities in the Berry connection when $\nabla_{\boldsymbol{\theta}}\alpha(\boldsymbol{\theta}) = \frac{h_1(\boldsymbol{\theta})\nabla_{\boldsymbol{\theta}} h_2(\boldsymbol{\theta}) - h_2(\boldsymbol{\theta})\nabla_{\boldsymbol{\theta}} h_1(\boldsymbol{\theta})}{h_1^2(\boldsymbol{\theta})+h_2^2(\boldsymbol{\theta})}$ is undefined; they occur at the critical points where $h_1(\boldsymbol{\theta}) = h_2(\boldsymbol{\theta}) = 0$.

Considering Eqs. 8 and 9 from the main text and taking $\delta = 0$, the values $h_1^{R,S}(\boldsymbol{\theta})$, $h_2^{R,S}(\boldsymbol{\theta})$, $h_3^{R,S}(\boldsymbol{\theta})$ are

$$\begin{aligned} h_1^{R,S}(\boldsymbol{\theta}) &= -\frac{\mu_b^{R,S} E_{21} \sin(\theta_1)}{2\sqrt{6}}, \\ h_2^{R,S}(\boldsymbol{\theta}) &= -\frac{\mu_a^{R,S} E_{32} \sin(\theta_2)}{4\sqrt{2}}, \\ h_3^{R,S}(\boldsymbol{\theta}) &= \frac{\mu_c^{R,S}}{2\sqrt{3}} E_{31}[m - \cos(\theta_1) - \cos(\theta_2)], \end{aligned} \tag{16}$$

and the aforementioned singularities occur at the $\boldsymbol{\theta} = (\theta_1, \theta_2)$ values $\boldsymbol{\theta}_{00} = (0,0)$, $\boldsymbol{\theta}_{0\pi} = (0,\pi)$, $\boldsymbol{\theta}_{\pi 0} = (\pi, 0)$, and $\boldsymbol{\theta}_{\pi\pi} = (\pi,\pi)$. Physically, these critical points indicate geometric conditions where certain components of light-matter coupling vanish.

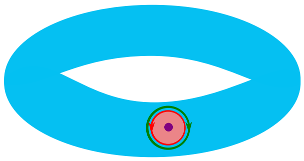

Figure 1: *Contour integration procedure to evaluate Chern number $C_l^{R,S}$.* The closed curve $\partial_r$ bounds both the pink region, which contains the singularity of $\boldsymbol{A}_l^{R,S}(\boldsymbol{\theta})$, and the blue region, which is rest of the torus. To apply Stokes theorem, we integrate counter-clockwise (red curve) along $\partial_r$ to find the surface integral for the pink region, and clockwise along $\partial_R$ (green curve) to find the surface integral for the blue region. The procedure can be extended to an arbitrary number of singularities of $\boldsymbol{A}_l^{R,S}(\boldsymbol{\theta})$.

The Chern number for the $R-$ and $S-$ enantiomer is proportional to the surface integral

of the corresponding Berry curvature over the torus $\mathbb{T}$,

$$C_l^{R,S} = \frac{1}{2\pi} \int\limits_{\mathbb{T}} d\boldsymbol{\theta} F_l^{R,S}(\boldsymbol{\theta}). \tag{17}$$

Using Stokes theorem, it can be written as a contour integral of the Berry connection; however, the singularities must be removed. To motivate the general procedure, first consider the case where the Berry connection $\boldsymbol{A}_l^{R,S}(\boldsymbol{\theta})$ contains only one singularity. The curve $\partial_r$ can be drawn, such that it defines an infinitesimal region containing the singularity (region I) and the rest of the torus (region II) (see Fig. 1). Applying a gauge transformation $|\epsilon_l^{R,S}(\boldsymbol{\theta})\rangle \rightarrow e^{i\phi_l^{R,S}(\boldsymbol{\theta})}|\epsilon_l^{R,S}(\boldsymbol{\theta})\rangle$ in region I can remove the singularity, $\boldsymbol{A}_l^{R,S}(\boldsymbol{\theta}) \rightarrow \boldsymbol{A'}_l^{R,S}(\boldsymbol{\theta}) = \boldsymbol{A}_l^{R,S}(\boldsymbol{\theta}) - \nabla_{\boldsymbol{\theta}}\phi_l^{R,S}(\boldsymbol{\theta})$, while the Berry curvature is unaffected[2,3]. Taking $\nabla_{\boldsymbol{\theta}}\phi_l^{R,S}(\boldsymbol{\theta}) = \boldsymbol{A}_l^{R,S}(\boldsymbol{\theta})$ achieves this desired result. The Chern numbers can then be written as the summation of contour integrals for each region:

$$\begin{aligned}
C_l^{R,S} &= \frac{1}{2\pi} \int\limits_{\mathbb{T}} d\boldsymbol{\theta} F_l^{R,S}(\boldsymbol{\theta}) \\
&= \frac{1}{2\pi} \oint\limits_{\partial_r} d\boldsymbol{\theta} \cdot \boldsymbol{A'}_l^{R,S}(\boldsymbol{\theta}) - \frac{1}{2\pi} \oint_{\partial_R} d\boldsymbol{\theta} \cdot \boldsymbol{A}_l^{R,S}(\boldsymbol{\theta}) \\
&= \frac{1}{2\pi} \oint\limits_{\partial_r} d\boldsymbol{\theta} \cdot [\boldsymbol{A}^{R,S}{}_l(\boldsymbol{\theta}) - \nabla_{\boldsymbol{\theta}}\phi_l^{R,S}(\boldsymbol{\theta})] - \frac{1}{2\pi} \oint_{\partial_R} d\boldsymbol{\theta} \cdot \boldsymbol{A}_l^{R,S}(\boldsymbol{\theta}) \\
&= -\frac{1}{2\pi} \oint\limits_{\partial_r} d\boldsymbol{\theta} \cdot \nabla_{\boldsymbol{\theta}}\phi_l^{R,S}(\boldsymbol{\theta}) \\
&= -\frac{1}{2\pi} \oint\limits_{\partial_r} d\boldsymbol{\theta} \cdot \boldsymbol{A}_l^{R,S}(\boldsymbol{\theta}).
\end{aligned} \tag{18}$$

In going from the first to the second line, we applied Stokes theorem in region I by traversing $\partial_r$ in a counterclockwise fashion, and in region II by doing so in a clockwise way (see Fig. 1).

If the Berry connection $\boldsymbol{A}_l^{R,S}(\boldsymbol{\theta})$ contains multiple singularities $\boldsymbol{\theta}_{ij}$, then local gauge transformations must be carried out in multiple regions to remove all of them. Then the

Chern number results in

$$C_l^{R,S} = -\sum_{ij} \frac{1}{2\pi} \oint_{\partial_{r_{ij}}} d\boldsymbol{\theta} \cdot \boldsymbol{A}_l^{R,S}(\boldsymbol{\theta}) \tag{19}$$

where the curves $\{\partial_{r_{ij}}\}$ enclose an infinitesimal region around each of the singularities $\boldsymbol{\theta}_{ij}$. Therefore, the Chern number can be calculated by studying the behavior of $\boldsymbol{A}_l^{R,S}(\boldsymbol{\theta})$ near the singularities.

Let $\boldsymbol{q} = (q_1, q_2)$ be a small displacement from the point $\boldsymbol{\theta}_{ij}$. Since $\sin(x) \approx x$ and $\sin(\pi + x) \approx -x$ as $x \to 0$, then

$$\begin{aligned}
\alpha^{R,S}(\boldsymbol{\theta}_{00} + \boldsymbol{q}) &\approx \beta^{R,S}, \\
\alpha^{R,S}(\boldsymbol{\theta}_{0\pi} + \boldsymbol{q}) &\approx -\beta^{R,S}, \\
\alpha^{R,S}(\boldsymbol{\theta}_{\pi 0} + \boldsymbol{q}) &\approx -\beta^{R,S}, \\
\alpha^{R,S}(\boldsymbol{\theta}_{\pi\pi} + \boldsymbol{q}) &\approx \beta^{R,S},
\end{aligned} \tag{20}$$

where $\tan \beta^{R,S} = \frac{\sqrt{3}\mu_a^{R,S} E_{32} q_2}{2\mu_b^{R,S} E_{21} q_1}$. The gradients $\nabla_{\boldsymbol{q}} \alpha^{R,S}(\boldsymbol{\theta})$ near the critical points can be readily evaluated in polar coordinates, $|\boldsymbol{q}| e^{i\gamma} = q_1 + i q_2$,

$$\begin{aligned}
\nabla_{\boldsymbol{q}} \alpha^{R,S}(\boldsymbol{\theta}_{00} + \boldsymbol{q}) &= -\nabla_{\boldsymbol{q}} \alpha^{R,S}(\boldsymbol{\theta}_{\pi 0} + \boldsymbol{q}) \\
&= -\nabla_{\boldsymbol{q}} \alpha^{R,S}(\boldsymbol{\theta}_{0\pi} + \boldsymbol{q}) \\
&= \nabla_{\boldsymbol{q}} \alpha^{R,S}(\boldsymbol{\theta}_{\pi\pi} + \boldsymbol{q}) \\
&\approx \frac{1}{|\boldsymbol{q}|} \frac{(\sqrt{3}\mu_a^{R,S} E_{32})(2\mu_b^{R,S} E_{21})}{(\sqrt{3}\mu_a^{R,S} E_{32})^2 \sin^2\gamma + (2\mu_b^{R,S} E_{21})^2 \cos^2\gamma} \hat{\boldsymbol{\gamma}}.
\end{aligned} \tag{21}$$

The line integral of $\nabla_{\boldsymbol{q}} \alpha^{R,S}(\boldsymbol{\theta}_{00} + \boldsymbol{q})$ over a small circle in the limit when $|\boldsymbol{q}| \to 0$,

$$
\begin{aligned}
&\oint_{|\boldsymbol{q}|\to 0} d\boldsymbol{q}\cdot\nabla_{\boldsymbol{q}}\alpha^{R,S}(\boldsymbol{\theta}_{00}+\boldsymbol{q})\\
=&\Big(\int_0^{\pi/2^-} d\gamma + \int_{\pi/2^+}^{3\pi/2^-} d\gamma\\
&+\int_{3\pi/2^+}^{2\pi} d\gamma\Big)\frac{(\sqrt{3}\mu_a^{R,S}E_{32})(2\mu E_{21})}{(\sqrt{3}\mu_a^{R,S}E_{32})^2\sin^2\gamma+(2\mu_b^{R,S}E_{21})^2\cos^2\gamma}\\
=&\Big(\int_0^{\mathrm{sgn}[(\mu_a^{R,S}E_{32})(\mu_b^{R,S}E_{21})]\infty} dx + \int_{-\mathrm{sgn}[(\mu_a^{R,S}E_{32})(\mu_b^{R,S}E_{21})]\infty}^{\mathrm{sgn}[(\mu_a^{R,S}E_{32})(\mu_b^{R,S}E_{21})]\infty} dx\\
&+\int_{-\mathrm{sgn}[(\mu_a^{R,S}E_{32})(\mu_b^{R,S}E_{21})]\infty}^{0} dx\Big)\frac{1}{1+x^2}\\
=&2\pi\mathrm{sgn}[(\mu_a^{R,S}E_{32})(\mu_b^{R,S}E_{21})]. \qquad (22)
\end{aligned}
$$

In the second line, we split the integral into three parts, noticing that the integral in the remaining infinitesimal regions around $\gamma=\pi/2$ and $\gamma=3\pi/2$ vanish given that the integrand is finite, $\int_{\pi/2^-}^{\pi/2^+} d\gamma(\cdot) = \int_{3\pi/2^-}^{3\pi/2^+} d\gamma(\cdot) = 0$. In the third line, we let $x = \frac{\sqrt{3}\mu_a^{R,S}E_{32}}{2\mu_b^{R,S}E_{21}}\tan\gamma$, and $dx = \frac{\sqrt{3}\mu_a^{R,S}E_{32}}{\mu_b^{R,S}E_{21}}\sec^2\gamma d\gamma$ and recognized that $x\to\mathrm{sgn}[(\mu_a^{R,S}E_{32})(\mu_b^{R,S}E_{21})]\infty$ as $\gamma\to(\pi/2)^-,(3\pi/2)^-$ and $x\to-\mathrm{sgn}[(\mu_a^{R,S}E_{32})(\mu_b^{R,S}E_{21})]\infty$ as $\gamma\to(\pi/2)^+,(3\pi/2)^+$.

The procedure of Eqs. (21) and (22) can be repeated for the other critical points, yielding,

$$
\begin{aligned}
&\oint_{|\boldsymbol{q}|\to 0} d\boldsymbol{q}\nabla_{\boldsymbol{q}}\alpha^{R,S}(\boldsymbol{\theta}_{0\pi}+\boldsymbol{q}) = -2\pi\mathrm{sgn}[(\mu_a^{R,S}E_{32})(\mu_b^{R,S}E_{21})],\\
&\oint_{|\boldsymbol{q}|\to 0} d\boldsymbol{q}\nabla_{\boldsymbol{q}}\alpha^{R,S}(\boldsymbol{\theta}_{\pi 0}+\boldsymbol{q}) = -2\pi\mathrm{sgn}[(\mu_a^{R,S}E_{32})(\mu_b^{R,S}E_{21})],\\
&\oint_{|\boldsymbol{q}|\to 0} d\boldsymbol{q}\nabla_{\boldsymbol{q}}\alpha^{R,S}(\boldsymbol{\theta}_{\pi\pi}+\boldsymbol{q}) = 2\pi\mathrm{sgn}[(\mu_a^{R,S}E_{32})(\mu_b^{R,S}E_{21})]. \qquad (23)
\end{aligned}
$$

Using Eqs. 15 and 19, the Chern number for the $l$-th band is

$$
\begin{aligned}
C_l^{R,S} &= -\sum_{ij} \frac{1}{2\pi} \oint_{\partial_{r_{ij}}} d\boldsymbol{\theta} \cdot \boldsymbol{A}_l^{R,S}(\boldsymbol{\theta}) \\
&= -\mathrm{sgn}[(\mu_a^{R,S} E_{21})(\mu_b^{R,S} E_{32})] \sum_{s=\pm 1} s[|c_{l,s}^{R,S}(\boldsymbol{\theta}_{00})|^2 - |c_{l,s}^{R,S}(\boldsymbol{\theta}_{0\pi})|^2 - |c_{l,s}^{R,S}(\boldsymbol{\theta}_{\pi 0})|^2 + |c_{l,s}^{R,S}(\boldsymbol{\theta}_{\pi\pi})|^2]
\end{aligned}
\tag{24}
$$

For $|m| < 2$ the Chern numbers for the upper, middle, and lower adiabatic states can be seen to yield,

$$
\begin{aligned}
C_U^{R,S} &= 2\mathrm{sgn}[m(\mu_a^{R,S} E_{32})(\mu_b^{R,S} E_{21})(\mu_c^{R,S} E_{31})], \\
C_M^{R,S} &= 0, \\
C_L^{R,S} &= -2\mathrm{sgn}[m(\mu_a^{R,S} E_{32})(\mu_b^{R,S} E_{21})(\mu_c^{R,S} E_{31})].
\end{aligned}
\tag{25}
$$

For $|m| > 2$, all $C_l^{R,S} = 0$. For the benefit of the reader, Table 1 provides an example calculation of the upper band Chern number $C_U^{R,S}$ for $|m| < 2$

Table 1: *Example Chern number calculation.* Shown are the values of the $|s = \pm 1\rangle$ amplitudes $|c_{U,s}^{R,S}(\boldsymbol{\theta}_{00})|^2$ for the upper band eigenstate at the singularity points $\boldsymbol{\theta}_{ij}$ for $|m| < 2$. Using these values and Eq. 24, we find that $C_U^{R,S} = 2\mathrm{sgn}[m(\mu_a^{R,S} E_{32})(\mu_b^{R,S} E_{21})(\mu_c^{R,S} E_{31})]$.

| | $\lvert c_{U,s}^{R,S}(\boldsymbol{\theta}_{00})\rvert^2$ | $\lvert c_{U,s}^{R,S}(\boldsymbol{\theta}_{0\pi})\rvert^2$ | $\lvert c_{U,s}^{R,S}(\boldsymbol{\theta}_{\pi 0})\rvert^2$ | $\lvert c_{U,s}^{R,S}(\boldsymbol{\theta}_{\pi\pi})\rvert^2$ |
|---|---|---|---|---|
| $s = 1$ | $\frac{1}{2} - \frac{1}{2}\mathrm{sgn}[(\mu_c^{R,S} E_{31})]$ | $\frac{1}{2} + \frac{1}{2}\mathrm{sgn}[m(\mu_c^{R,S} E_{31})]$ | $\frac{1}{2} + \frac{1}{2}\mathrm{sgn}[m(\mu_c^{R,S} E_{31})]$ | $\frac{1}{2} + \frac{1}{2}\mathrm{sgn}[(\mu_c^{R,S} E_{31})]$ |
| $s = -1$ | $\frac{1}{2} + \frac{1}{2}\mathrm{sgn}[(\mu_c^{R,S} E_{31})]$ | $\frac{1}{2} - \frac{1}{2}\mathrm{sgn}[m(\mu_c^{R,S} E_{31})]$ | $\frac{1}{2} - \frac{1}{2}\mathrm{sgn}[m(\mu_c^{R,S} E_{31})]$ | $\frac{1}{2} - \frac{1}{2}\mathrm{sgn}[(\mu_c^{R,S} E_{31})]$ |

# 5 Laser shot-noise

The laser shot noise is defined as the width of the photon distribution of the driving field. In the main text the laser field strength is assumed to be approximately $E = 10^{-9}$ a.u., or

$500\,\frac{\mathrm{V}}{\mathrm{m}}$. Assuming that the laser-beam waist area is $A = 1\mathrm{cm}^2$, its power is given by,

$$\begin{aligned} P &= \frac{cA\epsilon_0 E^2}{8\pi} \\ &= \frac{3\times 10^8\frac{\mathrm{m}}{\mathrm{s}} \times 1\,\mathrm{cm}^2 \times \frac{1\mathrm{m}^2}{100^2\mathrm{cm}^2} \times 8.85\times 10^{-12}\frac{\mathrm{C}^2}{\mathrm{J}\cdot\mathrm{m}} \times (500\frac{\mathrm{V}}{\mathrm{m}})^2}{8\pi} \\ &= 3\,\mathrm{mW} \end{aligned} \tag{26}$$

where $c$ is the speed of light and $\epsilon_0$ is the permittivity of free space. The frequencies of the molecular transitions in the main text are on the order of $v = 10\,\mathrm{GHz}$. Then the expected number of photons produced by the laser after a long enough time $t^* = 2000 \times 2\pi/\omega_2$ which guarantees TFC is

$$N = \frac{Pt^*}{hv} = \frac{3\times 10^{-3}\mathrm{W} \times 8 \times 10^{-3}\mathrm{s}}{6.63\times 10^{-34}\mathrm{J}\cdot\mathrm{s} \times 10 \times 10^9\mathrm{s}^{-1}} = 4\times 10^{18} \tag{27}$$

The photon distribution is taken to be Poissonian. The standard deviation of this distribution is $\sqrt{N}$, so the laser shot noise is $\sqrt{N} \sim 10^9$.

# References


(1) Simons, J. *An introduction to theoretical chemistry*; Cambridge University Press: Cambridge, 2003.

(2) Andrijauskas, T.; Anisimovas, E.; Račiūnas, M.; Mekys, A.; Kudriašov, V.; Spielman, I. B.; Juzeliūnas, G. Three-level Haldane-like model on a dice optical lattice. *Phys. Rev. A* **2015**, *92*, 033617.

(3) Goldman, N.; Anisimovas, E.; Gerbier, F.; Öhberg, P.; Spielman, I. B.; Juzeliūnas, G. Measuring topology in a laser-coupled honeycomb lattice: from Chern insulators to topological semi-metals. *New J. Phys.* **2013**, *15*, 013025.
